# Supplementary material for: Localization as an entanglement phase transition in boundary-driven Anderson models
Source: arXiv:1902.00025 source file (2019-07-23)
Supplement: Supplementary file 1 [file EntTrans_Supp.pdf]

# Localization as an entanglement phase transition in boundary-driven Anderson models: Supplementary Information

Michael J. Gullans and David A. Huse

*Department of Physics, Princeton University, Princeton, New Jersey 08544, USA*

(Dated: July 22, 2019)

## CONTENTS

|                                                |    |
|------------------------------------------------|----|
| S1. Scaling analysis for the mutual coherence  | S1 |
| S2. Cavity model for localized phase           | S3 |
| S3. Mutual coherence bounds mutual information | S5 |
| References                                     | S5 |

## S1. SCALING ANALYSIS FOR THE MUTUAL COHERENCE

In this section, we use qualitative arguments based on single-parameter scaling theory [S1] to derive the scaling behavior of the mutual coherence across the localization transition. Unlike the arguments based on the random quantum circuit model discussed in the main text, the formalism introduced in this section explicitly takes energy conservation into account. In principle, this formalism could be extended to derive the behavior in the entire critical regime  $\xi/L \sim 1$ ; however, for simplicity, we focus on the behavior in the two phases and at the critical point.

We can write a formula for the disorder averaged, non-equilibrium contribution to the mutual coherence as a double-energy integral over scattering states

$$\overline{C_d(A : B)} = \sum_{\mathbf{x} \in A, \mathbf{y} \in B} \overline{G_d(\mathbf{x}, \mathbf{y})} = \int dE \sum_{\mathbf{x} \in A, \mathbf{y} \in B} c_E^d(\mathbf{x}, \mathbf{y}) \int d\Delta f(E, \Delta), \quad (\text{S1})$$

$$c_E^d(\mathbf{x}, \mathbf{y}) = \overline{|q_E^d(\mathbf{x}, \mathbf{y})|^2}, \quad (\text{S2})$$

$$f(E, \Delta) = \frac{\sum_{\mathbf{x}, \mathbf{y}} [q_{E+\Delta/2}^d(\mathbf{x}, \mathbf{y})]^* q_{E-\Delta/2}^d(\mathbf{x}, \mathbf{y})}{\sum_{\mathbf{x} \in A, \mathbf{y} \in B} c_E^d(\mathbf{x}, \mathbf{y})}, \quad (\text{S3})$$

where  $c_E^d(\mathbf{x}, \mathbf{y})$  is the disorder average of  $|q_E^d(\mathbf{x}, \mathbf{y})|^2$  and  $f(E, \Delta)$  is an energy correlation function. This formulation is convenient because the energy-resolved spatial correlation functions  $q_E^{s,d}(\mathbf{x}, \mathbf{y})$  evolve under an Anderson model

$$-i\partial_t q_E^\alpha(\mathbf{x}, \mathbf{y}) = \sum_{\boldsymbol{\delta}} q_E^\alpha(\mathbf{x} + \boldsymbol{\delta}, \mathbf{y}) + (V_{\mathbf{x}} - E)q_E^\alpha(\mathbf{x}, \mathbf{y}), \quad (\text{S4})$$

where  $\boldsymbol{\delta}$  indexes nearest neighbor sites. This implies that  $c_E^d(\mathbf{x}, \mathbf{y})$  satisfies a diffusion equation for  $0 < W <$

$W_c$  [S2]

$$(i\omega + D_E \nabla_x^2) Y_E^D(\mathbf{x}, \mathbf{x}', \omega) = \delta(\mathbf{x} - \mathbf{x}'), \quad (\text{S5})$$

$$c_E^d(\mathbf{x}, \mathbf{y}) = \int d^3 x' |J_{E\mathbf{y}}^D(\mathbf{x}')|^2 Y_E^D(\mathbf{x}, \mathbf{x}', 0), \quad (\text{S6})$$

$$Y_E^D(\mathbf{x}, \mathbf{x}', \omega) = \overline{G_{E+\omega/2}^A(\mathbf{x}, \mathbf{x}') G_{E-\omega/2}^R(\mathbf{x}, \mathbf{x}')}, \quad (\text{S7})$$

where  $|J_{E\mathbf{y}}^D(\mathbf{x}')|^2$  is an effective DC source term centered near  $\mathbf{x}' = \mathbf{y}$  and  $Y_E^D(\mathbf{x}, \mathbf{x}', \omega)$  is the disorder averaged density-density response function on the diffusive length scale ( $G_E^{A/R}$  are the retarded/advanced Green's functions). Since there is no diffusion in the leads,  $Y_E^D(\mathbf{x}, \mathbf{x}', \omega)$  has to satisfy the boundary condition that it vanishes in the leads [S2]. As a result, this equation will have the solution

$$Y_E^D(\mathbf{x}, \mathbf{x}', 0) = \frac{1}{4\pi D_E |\mathbf{x} - \mathbf{x}'|} + V_{\mathbf{x}'}^D(\mathbf{x}), \quad |\mathbf{x} - \mathbf{x}'| \gg \xi, \quad (\text{S8})$$

where  $\xi \sim |W - W_c|^\nu$  is the correlation length on the diffusive side and  $V_{\mathbf{x}'}^D(\mathbf{x})$  is non-singular at  $\mathbf{x} = \mathbf{x}'$  and is chosen to satisfy the boundary conditions.

At a given energy there are strong fluctuations in both the density gradient and local current, which means that the source term for the non-equilibrium density will simply scale as the difference in the Fermi functions,  $|J_{E\mathbf{y}}^D(\mathbf{x}')|^2 \sim [n_E^d]^2 = (n_E^L - n_E^R)^2$ ; however, the diffusive description is only valid for  $|\mathbf{x} - \mathbf{x}'|$  much greater than the correlation length  $\xi$ , whereas the scaling  $c_E^d(\mathbf{x}, \mathbf{y}) \sim [n_E^d]^2$  only holds on lengths scales on the order of the mean free path  $\ell$ . To match the two scales  $\ell < |\mathbf{x} - \mathbf{y}| < \xi$ , we use the approximate description of the critical regime in terms of a scale dependent diffusion constant [S1]

$$\vec{\nabla}_x \cdot D_c(\mathbf{x} - \mathbf{x}') \vec{\nabla}_x Y_E^c(\mathbf{x}, \mathbf{x}', 0) = \delta(\mathbf{x} - \mathbf{x}'), \quad (\text{S9})$$

where  $D_c(\mathbf{x} - \mathbf{x}') \sim |\mathbf{x} - \mathbf{x}'|^{2-d_0}$  for spatial dimension  $d_0$ . The solution to this anomalous diffusion equation in the absence of boundaries is scale-invariant, which can be seen by rescaling space  $\mathbf{x} \rightarrow \alpha \mathbf{x}$ . Integrating both sides of Eq. (S9) over a ball of radius  $\epsilon$  and applying Green's theorem in the limit  $\epsilon \rightarrow 0$  we find

$$Y_E^c(\mathbf{x}, \mathbf{x}', 0) = -\frac{1}{4\pi} \log(|\mathbf{x} - \mathbf{x}'|) + V_{\mathbf{x}'}^c(\mathbf{x}), \quad (\text{S10})$$

where  $V_{\mathbf{x}'}^c(\mathbf{x})$  is non-singular at  $\mathbf{x} = \mathbf{x}'$  and is needed to match the boundary conditions on  $Y_E^c$  away from the source. The solution for the coherence field will then be given by

$$c_E^d(\mathbf{x}, \mathbf{y}) = \int d^3 x' |J_{E\mathbf{y}}^c(\mathbf{x}')|^2 Y_E^c(\mathbf{x}, \mathbf{x}', 0), \quad \xi > |\mathbf{x} - \mathbf{y}| \gg \ell. \quad (\text{S11})$$

Finally, in the vicinity of  $|\mathbf{x} - \mathbf{y}| \gtrsim \ell$ , the diffusion constant saturates to its microscopic value  $D_{0E} = v_F \ell / d_0$  where  $v_F$  is the Fermi velocity. The solution in the critical regime has the property that the amplitude of  $c_E^d(\mathbf{x}, \mathbf{y})$  is independent of the length scale, which implies that it inherits the scaling  $[n_E^d]^2$  from the microscopic regime. Matching this scaling to the diffusive region we arrive at the result

$$c_E^d(\mathbf{x}, \mathbf{y}) \sim \frac{\xi [n_E^d]^2}{|\mathbf{x} - \mathbf{y}|}, \quad L_0 \gg |\mathbf{x} - \mathbf{y}| \gtrsim \xi. \quad (\text{S12})$$

The functional form for separations on the order of  $L_0$  can be found by solving the diffusion equation with the appropriate boundary conditions at the leads, which inherits the scaling of Eq. (S12).

The mutual coherence also depends on the energy correlation function; however, this correlation function will only have significant correlations on the scale of the Thouless energy  $E_{\text{Th}} = D/L_0^2$ . Assuming this scaling, and using the fact that  $D \sim 1/\xi$ , we arrive at an overall volume law scaling for the mutual coherence in the low-temperature regime  $T \ll \delta\mu$  that is independent of  $\xi$

$$C_d(L : R) \sim \int dE [n_E^d]^2 L_0^3 \sim |\delta\mu| L_0^3. \quad (\text{S13})$$

At the critical point ( $\xi \rightarrow \infty$ ) there is no diffusive region and  $c_E^d(\mathbf{x}, \mathbf{y})$  maintains an amplitude on the order of  $[n_E^d]^2$  throughout the entire sample. On the other hand, the Thouless energy is reduced to scale as the level spacing  $E_{\text{Th}} \sim 1/L_0^3$  because that is the transit time through the sample in the presence of the anomalous diffusion. In this case, we still find a volume law scaling for the mutual coherence, but its precise prefactor will differ from the diffusive phase

$$C_d(L : R) \sim |\delta\mu|L_0^3. \quad (\text{S14})$$

This scaling will persist until  $\delta\mu$  approaches the mobility edge.

For the resonant states in the insulating phase  $W > W_c$ , the coherence field remains localized in the region  $|\mathbf{x} - \mathbf{y}| \lesssim \xi$  with amplitude on the order of  $[n_E^d]^2$ , which strongly reduces the total amount of mutual coherence. The energy correlation range is, however, much larger. A sensible upper bound is to use the level spacing in the localized region  $\sim 1/\xi^3$ . Together these two scalings predict the upper bound for the scaling for the mutual coherence in the localized phase

$$C_d(L : R) \lesssim |\delta\mu|\xi L_0^2. \quad (\text{S15})$$

## S2. CAVITY MODEL FOR LOCALIZED PHASE

In this section, we present a simplified cavity model to describe the mutual coherence in the localized phase. Transport in the localized phase occurs through “resonant” states in the sample that have exponentially small, but nearly equal, tunneling rates to both leads. These states give rise to narrow transmission peaks, whose width is much less than the single-particle level spacing in the sample  $\sim L_0^{-3}$ .

Since many qualitative aspects of the localized phase in 3D are present already in 1D, we consider a 1D model of the form

$$\begin{aligned} H &= \sum_{x < 0, x > L_0} (c_x^\dagger c_{x+1} + h.c.) + t_L(c_0^\dagger c_1 + h.c.) + t_R(c_{L_0}^\dagger c_{L_0+1} + h.c.) + \sum_n \omega_n b_n^\dagger b_n \\ &= \sum_{x < 0, x > L_0} t(c_x^\dagger c_{x+1} + h.c.) + \sum_n (t_L \phi_1^n b_n^\dagger c_0 + t_R \phi_{L_0}^n b_n^\dagger c_{L_0+1} + h.c.) + \sum_n \omega_n b_n^\dagger b_n, \end{aligned} \quad (\text{S16})$$

where  $c_x$  are fermion operators on an infinite lattice, the sample consists of sites  $1, \dots, L_0$ , with local tunneling rates  $t_{L/R}$  to the left/right lead (taken to be exponentially small in analogy to the resonant states), and  $b_n = \sum_x \phi_x^n c_x$  are operators that create eigenstates of the sample when  $t_L = t_R = 0$  with energies  $\omega_n$ . For a disordered system,  $\phi_x^n$  are the localized wavefunctions, but they could also be eigenstates of a finite chain with hopping  $t_0$ , in which case

$$\omega_n = 2t_0 \cos[n\pi/(L_0 + 1)], \quad n = 1, \dots, L_0, \quad (\text{S17})$$

$$\phi_x^n \propto \sin[nx\pi/(L_0 + 1)], \quad x = 1, \dots, L_0. \quad (\text{S18})$$

This effectively models a Fabrey-Perot cavity. The scattering state wavefunctions can be found from Schrödinger's equation

$$\epsilon_k \psi_0^k = \psi_{-1}^k + t_L \sum_n \phi_1^n \psi_n^k, \quad (\text{S19})$$

$$\epsilon_k \psi_n^k = t_L \phi_1^n \psi_0^k + \omega_n \psi_n^k + t_R \phi_{L_0}^n \psi_{L_0+1}^k, \quad (\text{S20})$$

$$\epsilon_k \psi_{L_0+1}^k = \psi_{L_0+2}^k + t_R \sum_n \phi_{L_0}^n \psi_n^k, \quad (\text{S21})$$

where  $\epsilon_k = 2 \cos k$  is the energy of a scattering state in the lead with wavefunctions  $e^{\pm i k x}$ . Assuming  $\epsilon_k = \omega_{n_0}$

for a given  $n_0$ , we find the solution

$$\psi_{L_0+1}^k = -\frac{t_L \phi_1^{n_0}}{t_R \phi_{L_0}^{n_0}} \psi_0^k, \quad (\text{S22})$$

$$\psi_n^k = \frac{t_L}{\epsilon_k - \omega_n} \left( \phi_1^n - \phi_{L_0}^n \frac{\phi_1^{n_0}}{\phi_{L_0}^{n_0}} \right) \psi_0^k, \quad (\text{S23})$$

$$\psi_{n_0}^k = \frac{e^{-ik}}{t_L \phi_1^{n_0}} \psi_0^k - \sum_{n \neq n_0} \frac{t_L \phi_1^n}{\epsilon_k - \omega_n} \left( \phi_1^n - \phi_{L_0}^n \frac{\phi_1^{n_0}}{\phi_{L_0}^{n_0}} \right) \frac{\psi_0^k}{\phi_1^{n_0}}, \quad (\text{S24})$$

$$\psi_{L_0+2}^k = \epsilon_k \psi_{L_0+1}^k - t_R \sum_n \phi_{L_0}^n \psi_n^k. \quad (\text{S25})$$

The transmission coefficient for a state incoming from the right lead is given by

$$t_k^- = \frac{2i \sin k}{\psi_{L_0+1}^k - e^{-ik} \psi_{L_0+2}^k}, \quad (\text{S26})$$

evaluated for  $\psi_0^k = 1$ . The solution to the right incoming scattering state wavefunction is then given by Eqs. (S22) and (S25) with  $\psi_0^k = t_k^-$ . In the vicinity of a resonance, for  $t_L^2, t_R^2$  and  $\delta = \omega_{n_0} - \epsilon_k$  much less than the level spacing in the sample, the transmission coefficient is approximately given by

$$t_k^- \approx \frac{2i \sin k e^{2ik} \phi_1^{n_0} \phi_{L_0}^{n_0} t_L t_R}{\phi_1^{n_0 2} t_L^2 + \phi_{L_0}^{n_0 2} t_R^2 - \delta e^{ik}}. \quad (\text{S27})$$

This corresponds to a Lorentzian profile about the resonance with a width given by the same result one obtains from a Fermi's golden rule calculation

$$\gamma_{n_0} = (\phi_1^{n_0 2} t_L^2 + \phi_{L_0}^{n_0 2} t_R^2) \sin^2 k. \quad (\text{S28})$$

The behavior of the current and density gradient in this cavity model is more subtle because one also has to take into account the exponentially suppressed amplitude of the off-resonant states. We can gain some intuition for the properties of this solution by considering a two-site system with  $n_0 = 1$ . In this case, the expectation value of the current and density gradient in the scattering state from the right lead with energy  $\epsilon_k$  are given by

$$J_k^R = i \langle 0 | a_{\epsilon_k}^R (c_1^\dagger c_2 - c_2^\dagger c_1) a_{\epsilon_k}^{R\dagger} | 0 \rangle \propto 2(\phi_1^1 \phi_2^2 - \phi_2^1 \phi_1^2) \text{Im}[\psi_1^{k*} \psi_2^k], \quad (\text{S29})$$

$$\nabla n_k^R = \langle 0 | a_{\epsilon_k}^R (c_1^\dagger c_1 - c_2^\dagger c_2) a_{\epsilon_k}^{R\dagger} | 0 \rangle \propto 2(\phi_1^1 \phi_1^2 - \phi_2^1 \phi_2^2) \text{Re}[\psi_1^{k*} \psi_2^k]. \quad (\text{S30})$$

For a two mode system without disorder, one mode is symmetric and the other is anti-symmetric, implying that the wavefunction coefficient is non-zero. From these expressions we can determine that the current and density gradient on resonance both scale as  $|t_k^-|^2 \sim 1$  when  $t_L \sim t_R$ . On the other hand, the coherence between the two sites actually diverges as

$$\langle 0 | a_{\epsilon_k}^R c_1^\dagger c_2 a_{\epsilon_k}^{R\dagger} | 0 \rangle \propto \phi_1^1 \phi_2^1 |\psi_1^k|^2 \sim 1/t_{L/R}^2. \quad (\text{S31})$$

This implies that after summing over the scattering states in the vicinity of the resonance, which has a width  $\gamma_1 \sim t_{L/R}^2$ , one finds that  $J \cdot \nabla n \sim t_{L/R}^2$  and  $\langle c_1^\dagger c_2 \rangle \sim 1$ . This is consistent with our intuitive picture that the coherences are sourced at an exponentially slow rate, but live for an exponentially long time, leading to an order one coherence density within each resonant localized state. The contribution to the current and mutual coherence from scattering states that are far detuned in energy from the resonant states is exponentially suppressed.

### S3. MUTUAL COHERENCE BOUNDS MUTUAL INFORMATION

In this section, we show that the mutual coherence serves as a generic lower bound to the mutual information for Gaussian fermionic states. Near infinite temperature, the mutual coherence approximates the mutual information and the fermionic entanglement negativity [S3].

The Renyi entropies can be expressed in terms of the correlation matrix  $G$  as

$$S_\alpha(\rho) = \frac{1}{1-\alpha} \log \text{Tr}[\rho^\alpha] = \frac{1}{1-\alpha} \text{Tr}[\log(G^\alpha + (\mathbb{I} - G)^\alpha)], \quad \alpha \neq 1, \quad (\text{S32})$$

$$S_1(\rho) = -\text{Tr}[\rho \log \rho] = -\text{Tr}[G \log G] - \text{Tr}[(\mathbb{I} - G) \log(\mathbb{I} - G)], \quad (\text{S33})$$

where  $G_{ij} = \text{Tr}[\rho c_i^\dagger c_j]$  and the second equality in Eq. (S32) and Eq. (S33) holds for Gaussian fermionic states that conserve particle number. To prove the bound on the mutual information  $I_1(A : B) = S_1(\rho_A) + S_1(\rho_B) - S_1(\rho_{AB})$ , we first transform into a basis where  $G$  is diagonal in subspace  $A$  and  $B$ , i.e.,

$$UGU^\dagger = D + c, \quad (\text{S34})$$

$$D = \begin{pmatrix} D_A & 0 \\ 0 & D_B \end{pmatrix}, \quad (\text{S35})$$

where  $D$  is a diagonal matrix with eigenvalues between 0 and 1 and  $c$  is only nonzero in the upper and lower right blocks.

We define the particle number  $N_{AB}^p = \text{Tr}[D]$  and hole number  $N_{AB}^h = N_{AB} - N_{AB}^p$ , where  $N_{AB}$  is the total number of sites in  $A$  and  $B$ . We introduce the single-particle/hole density matrices (i.e., positive, semidefinite Hermitian matrices with unit trace)  $\rho^p = (D + c)/N_{AB}^p$  and  $\rho^h = (\mathbb{I} - D - c)/N_{AB}^h$  and the diagonal density matrices  $\rho_d^p = D/N_{AB}^p$  and  $\rho_d^h = (\mathbb{I} - D)/N_{AB}^h$ . The mutual information can be written as the sum of relative entropies in this  $N_{AB}$ -dimensional Hilbert space

$$I_1(A : B) = N_{AB}^p S(\rho^p | \rho_d^p) + N_{AB}^h S(\rho^h | \rho_d^h), \quad (\text{S36})$$

where the relative entropy is defined as  $S(\rho | \sigma) = -\text{Tr}[\rho \log \sigma] - S_1(\rho)$ . Using the bound on the relative entropy  $S(\rho | \sigma) \geq \frac{1}{2} \|\rho - \sigma\|_1^2$  and the inequality  $\|X\|_1 \geq \text{Tr}[XY]/\|Y\|$  [S5], we arrive at the bounds

$$N_{AB}^a S(\rho^a | \rho_d^a) \geq \frac{1}{2N_{AB}^a} \left( \frac{\text{Tr}[cG]}{\|G\|} \right)^2 = \frac{1}{2N_{AB}^a} \left( \frac{\text{Tr}[c^2]}{\|G\|} \right)^2 \geq \frac{C(A : B)^2}{2N_{AB}^a}. \quad (\text{S37})$$

Together, these two inequalities imply the lower bound

$$I_1(A : B) \geq \frac{N_{AB}}{2N_{AB}^p N_{AB}^h} C(A : B)^2. \quad (\text{S38})$$

As a result, when  $N_{AB}^{p/h}$  and  $C(A : B)$  are all extensive quantities (i.e., proportional to  $N_{AB}$ ), then the mutual information must also be extensive.

One limit where  $C(A : B)$  is directly proportional to the mutual information is when the fermionic system is close to an infinite temperature state with  $G = \frac{\mathbb{I}}{2} + \delta G$ . Expanding in powers of  $\delta G$  for any  $\alpha > 0$ , we find

$$S_\alpha(\rho) = N \log 2 - 2\alpha \text{Tr}[\delta G^2] + O(\text{Tr}[\delta G^3]), \quad (\text{S39})$$

$$I_1(A : B) = 2C(A : B). \quad (\text{S40})$$

Using identities proved in [S6], one can show that the fermionic entanglement negativity [S3] can also be approximated in terms of the mutual coherence when the system is near infinite temperature.

---

[S1] J. T. Chalker, *Scaling and eigenfunction correlations near a mobility edge*, Physica A **167**, 253 (1990).

- [S2] K. Efetov, *Supersymmetry in Disorder and Chaos*, Ch. 9.1, (Cambridge University Press, Cambridge, UK, 1999).
- [S3] H. Shapourian and S. Ryu, *Entanglement negativity of fermions: Monotonicity, separability criterion, and classification of few-mode states*, Phys. Rev. A **99**, 022310 (2019).
- [S4] M.-C. Bañuls, J. I. Cirac, and M. M. Wolf, *Entanglement in fermionic systems*, Phys. Rev. A **76**, 022311 (2007).
- [S5] M. M. Wolf, F. Verstraete, M. B. Hastings, and J. I. Cirac, *Area laws in quantum systems: Mutual information and correlations*, Phys. Rev. Lett. **100**, 070502 (2008).
- [S6] J. Eisert, V. Eisler, and Z. Zimborás, *Entanglement negativity bounds for fermionic gaussian states*, Phys. Rev. B **97**, 165123 (2018).
